# Supplementary material for: Small-scale displacement fluctuations of vesicles in fibroblasts
Source: arXiv:1803.06013 ancillary file (2018-08-16)
Supplement: Supplementary file 1 [file SM_PDF.pdf]

# Small-scale displacement fluctuations of vesicles in fibroblasts

Danielle Posey<sup>1</sup>, Paris Blaisdell-Pijuan<sup>2</sup>, Samantha K. Knoll<sup>3</sup>, Taher A. Saif<sup>3</sup>, and Wylie W. Ahmed<sup>2,\*</sup>

<sup>1</sup>Department of Biological Sciences, California State University, Fullerton, CA

<sup>2</sup>Department of Physics, California State University, Fullerton, CA <sup>3</sup>Department of Mechanical Science and Engineering, University of Illinois, Urbana, IL <sup>\*</sup>Corresponding author (wahmed@fullerton.edu)

## Supplementary Material

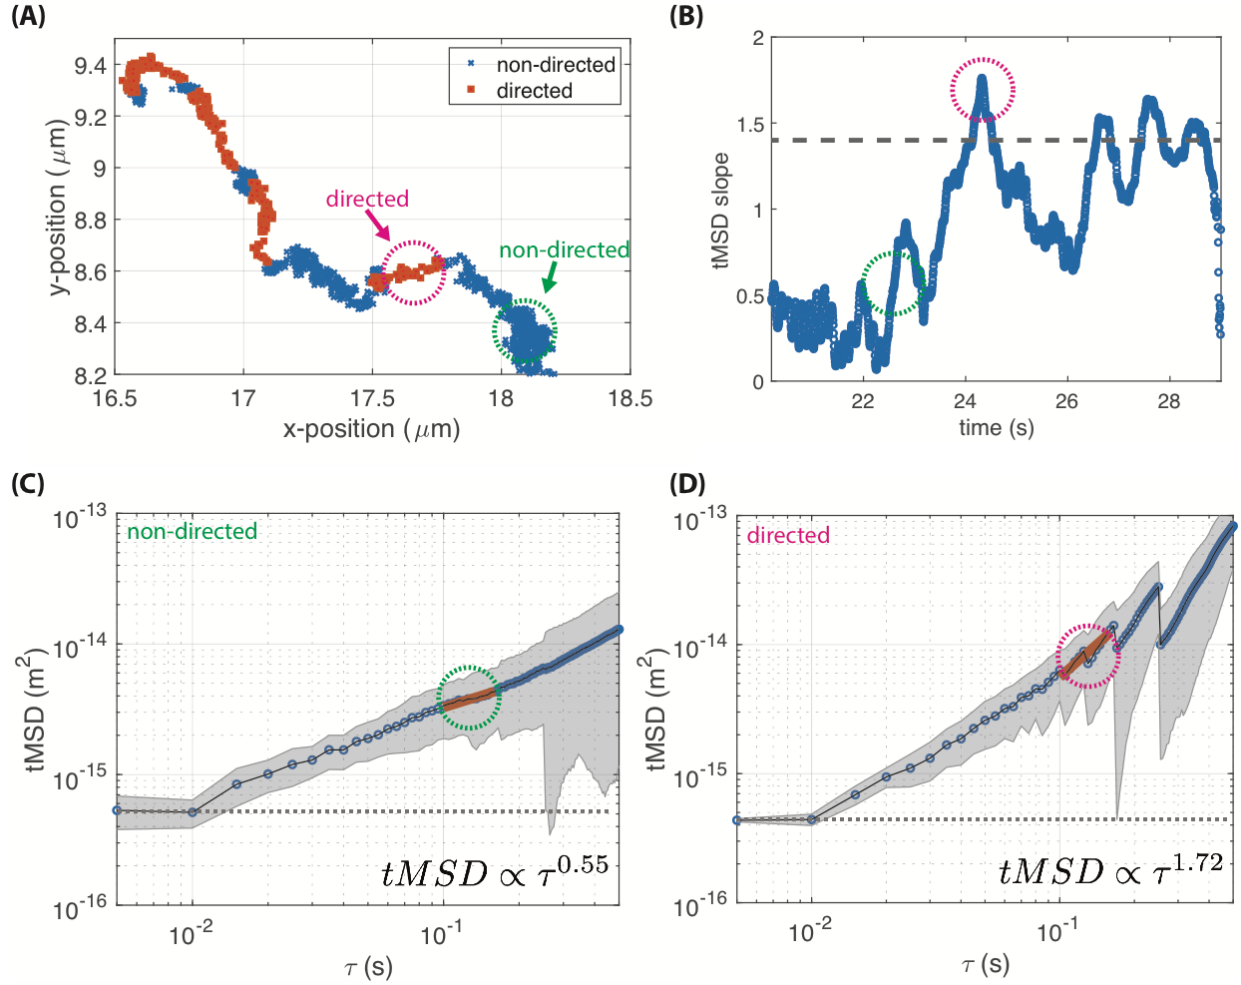

**Figure S1:** (A) A representative trajectory of a vesicle indicating directed (squares) and non-directed (x) motion. The circled regions for directed (magenta) and non-directed (green) correspond to the circled data in B, C, and D. (B) The power-law of the tMSD analysis plotted as a function of time. (C) A representative tMSD of a vesicle undergoing non-directed motion with a sub-diffusive power-law of 0.55. The horizontal dashed line indicates the tracking uncertainty ( $\sim 23$  nm). (D) A representative tMSD of a vesicle undergoing directed motion with a super-diffusive power-law of 1.72. The horizontal dashed line indicates the tracking uncertainty ( $\sim 21$  nm). As evidenced by (C) and (D), the tMSD analysis is well-above the tracking uncertainty. (shaded gray region indicates standard deviation)

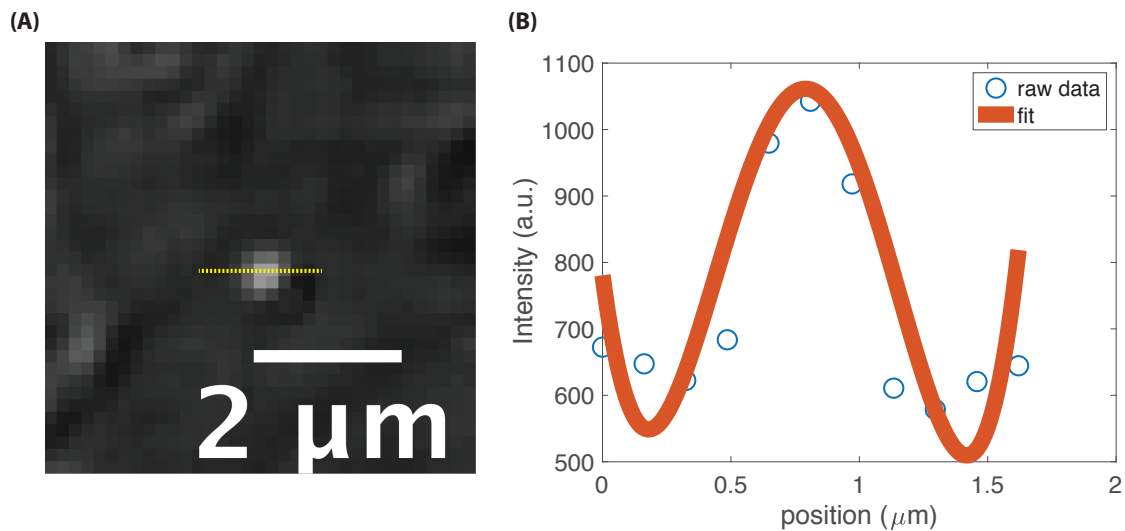

**Figure S2:** (A) A representative differential interference contrast (DIC) microscopy image of a vesicle in a fibroblast. Horizontal dashed yellow line indicates the region of intensity measurements for fitting. (B) Example of raw intensity data (circles) with a polynomial fitting with Gaussian weight (solid line) indicating the algorithm developed by Rogers et al. *Physical Biology* 2007 is able to fit particles in DIC images.
